# Supplementary material for: CdSe Colloidal Quantum Rings
Source: arXiv:1509.07793 ancillary file (2015-09-28)
Supplement: Supplementary file 1 [file Supplementary_Materials.pdf]

# Supporting information for: CdSe Colloidal Quantum Rings

Sébastien A. Lamarre,[†,‡] Étienne Rochette,[†,‡] Samuel Tremblay,[¶,‡] and Claudine Nì. Allen*,[¶,‡]

*Département de chimie, Université Laval, Québec, G1V 0A6, Canada, Centre d'optique, photonique et laser (COPL), and Département de physique, de génie physique et d'optique, Université Laval, Québec, G1V 0A6, Canada*

E-mail: claudine.allen@phy.ulaval.ca

*To whom correspondence should be addressed
[†]Département de chimie, Université Laval, Québec, G1V 0A6, Canada
[‡]Centre d'optique, photonique et laser (COPL)
[¶]Département de physique, de génie physique et d'optique, Université Laval, Québec, G1V 0A6, Canada

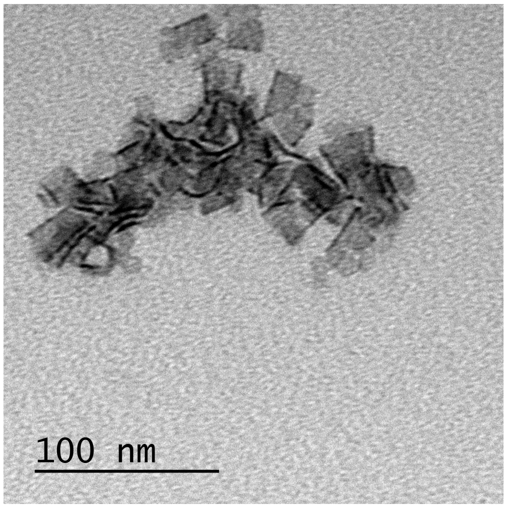


Figure S1: Transmission electron microscopy image of 3 ML cQRs with 5 $\mu$mol of Se.

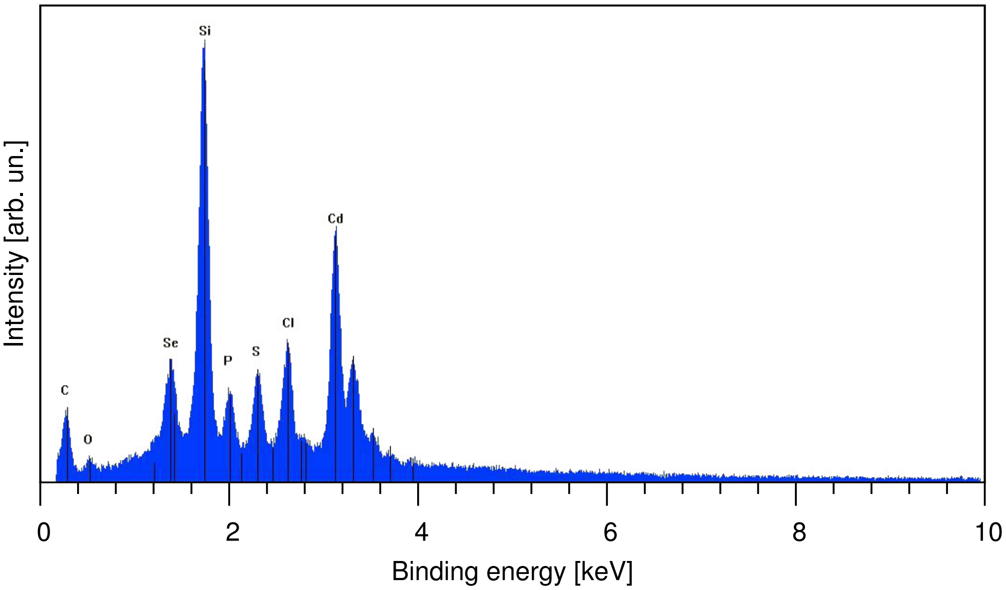


Figure S2: Example energy dispersive X-ray spectrum of 3 ML cQRs with 100 $\mu$mol of Se.

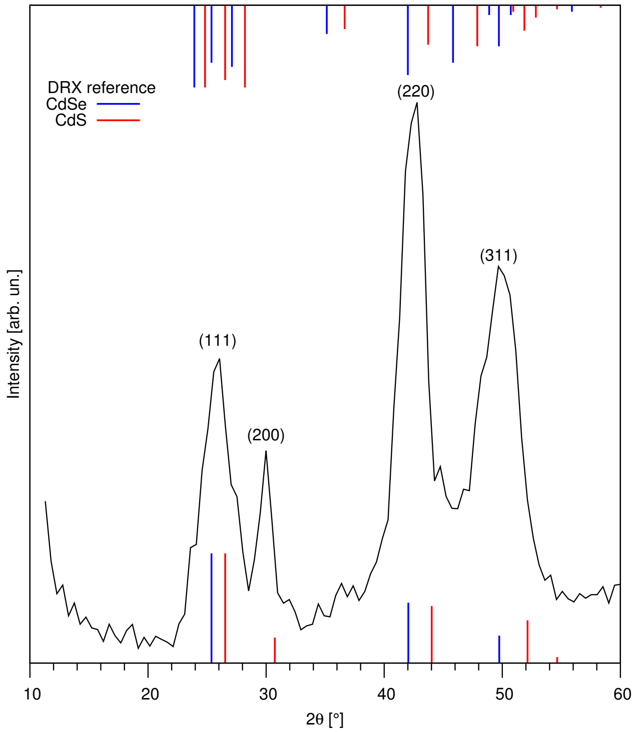


Figure S3: X-ray diffraction pattern of 3 ML cQRs with 100 $\mu$mol of Se. The peaks are labeled with the diffraction peaks for the zinc blende phase. As reference, zinc blende pattern of CdS (AMCSD 70) and CdSe (JCPDS 19-191) are presented at the bottom and wurtzite pattern of CdS (JCPDS 41-1049) and CdSe (JCPDS 8-459) at the top.

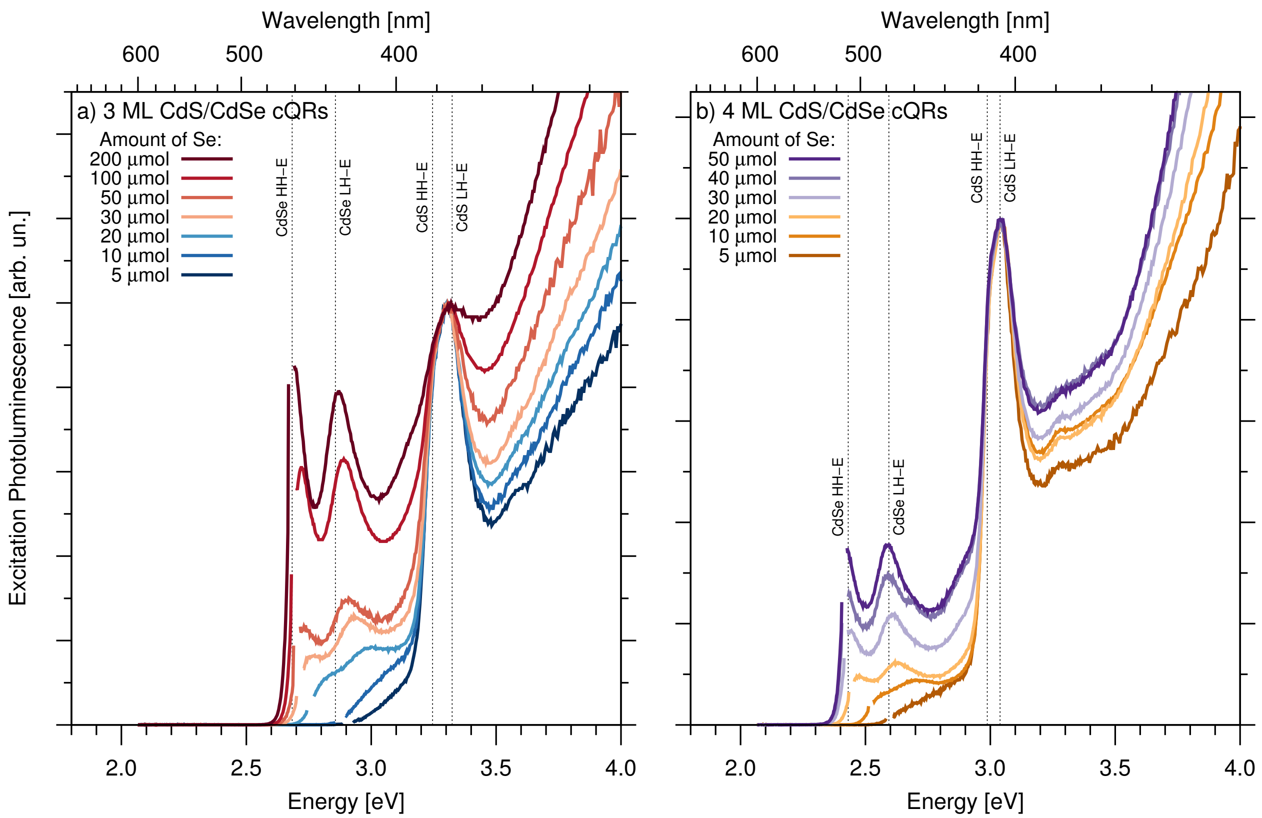


Figure S4: Photoluminescence excitation spectra of (a) 3 ML and (b) 4 ML cQRs samples. The transitions are labeled 1) CdSe HH-E, 2) CdSe LH-E, 3) CdS HH-E and 4) CdS LH-E. The spectra are normalized by the CdS NPL absorption transition.

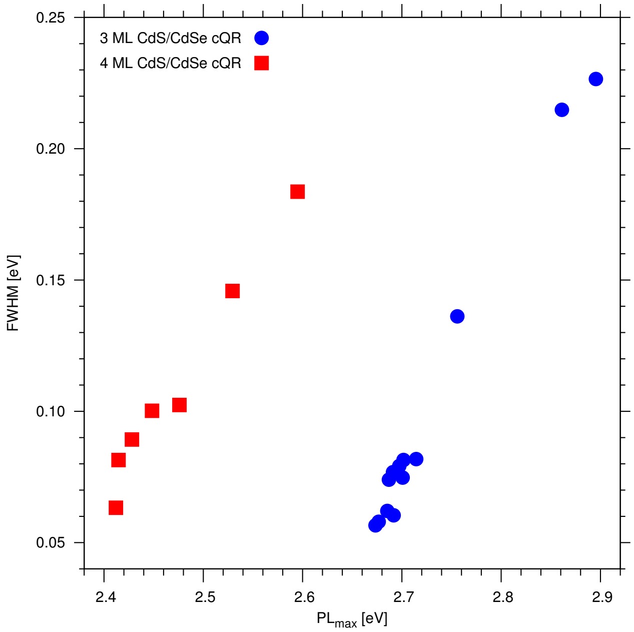


Figure S5: Relation between the $PL_{max}$ and its FWHM for all samples of each thickness.
